# Supplementary material for: Quantitative disentanglement of spin Seebeck, proximity-induced and intrinsic anomalous Nernst effect in NM/FM bilayers
Source: arXiv:1702.05384 ancillary file (2017-02-16)
Supplement: Supplementary file 1 [file Panagiota_Bougiatioti_Supplementary_Materials.pdf]

## - Supplemental Materials -

### Quantitative disentanglement of spin Seebeck, proximity-induced and intrinsic anomalous Nernst effect in NM/FM bilayers

Panagiota Bougiatioti<sup>1</sup>, Christoph Klewe<sup>1,2</sup>, Daniel Meier<sup>1</sup>, Orestis Manos<sup>1</sup>, Olga Kuschel<sup>3</sup>, Joachim Wollschläger<sup>3</sup>, Laurence Bouchenoire<sup>4,5</sup>, Simon D. Brown<sup>4,5</sup>, Jan-Michael Schmalhorst<sup>1</sup>, Günter Reiss<sup>1</sup>, and Timo Kuschel<sup>1,6</sup>

<sup>1</sup>*Center for Spinelectronic Materials and Devices, Department of Physics, Bielefeld University, Universitätsstraße 25, 33615 Bielefeld, Germany*

<sup>2</sup>*Advanced Light Source, Lawrence Berkeley National Laboratory, Berkeley, CA 94720, USA*

<sup>3</sup>*Department of Physics and Center of Physics and Chemistry of New Materials, Osnabrück University, Barbarastrasse 7, 49076 Osnabrück, Germany*

<sup>4</sup>*XMaS, European Synchrotron Radiation Facility, Grenoble, 38043, France*

<sup>5</sup>*Department of Physics, University of Liverpool, Liverpool L69 7ZE, UK*

<sup>6</sup>*Physics of Nanodevices, Zernike Institute for Advanced Materials, University of Groningen, Nijenborgh 4, 9747 AG Groningen, The Netherlands*

(Dated: February 15, 2017)

#### I. SAMPLE FABRICATION

We fabricated thin films by reactive sputter deposition [1] starting from pure high-resistive  $\text{NiFe}_2\text{O}_4$  (NFO) ( $\sim 160$  nm) up to the metallic  $\text{Ni}_{33}\text{Fe}_{67}$  (10.4 nm) with intermediate  $\text{NiFe}_2\text{O}_{x_1}$  (60 nm) and  $\text{NiFe}_2\text{O}_{x_2}$  (35 nm), with  $4 > x_1 > x_2 > 0$ . The films were deposited on  $\text{MgAl}_2\text{O}_4(001)$  (MAO) substrates by dc magnetron sputtering. The metallic film was deposited in Ar atmosphere with pressure in the range of  $2 \cdot 10^{-3}$  mbar at room temperature (RT). The  $\text{NiFe}_2\text{O}_{x_1}$  and  $\text{NiFe}_2\text{O}_{x_2}$  films were prepared by reactive co-sputtering from an elemental Ni and Fe target in Ar and  $\text{O}_2$  atmosphere at  $610^\circ\text{C}$  substrate temperature. For the  $\text{NiFe}_2\text{O}_{x_1}$  bilayer the Ar partial pressure during the deposition was  $1.7 \cdot 10^{-3}$  mbar, while the total pressure was  $2 \cdot 10^{-3}$  mbar. For the  $\text{NiFe}_2\text{O}_{x_2}$  bilayer the Ar partial pressure was  $1.8 \cdot 10^{-3}$  mbar, while the total pressure was  $2.3 \cdot 10^{-3}$  mbar. The pure NFO was grown in pure  $\text{O}_2$  atmosphere with a pressure of  $2 \cdot 10^{-3}$  mbar at  $610^\circ\text{C}$  substrate temperature. The base pressure in all cases was less than  $10^{-8}$  mbar.

#### II. THEORETICAL AND EXPERIMENTAL BACKGROUND FOR XRMR

A fundamental theoretical background for the XRMR includes the determination of the optical properties of a material exposed to x-rays as given in the refractive index  $n = 1 - \delta + i\beta$ , where  $\delta$  and  $\beta$  are the dispersion and the absorption coefficients, respectively, connected via the Kramers-Kronig relation. When the magnetization changes directions ( $\pm$ ), the optical parameters  $\delta$  and  $\beta$  vary by a fraction  $\Delta\delta$  and  $\Delta\beta$ , respectively. These so called magneto-optical parameters are most pronounced at energies right around the absorption edge of the investigated material and vanish far from the resonance. Considering the interference of the reflected light from the surface and the interfaces this method can reveal a possible spin polarization in a film independent from the layer thickness [2].

Here, the XRMR data were collected at a fixed energy close to the Pt  $L_3$  absorption edge by performing x-ray reflectivity (XRR) scans with circularly polarized x-rays (off-resonant at 11465 eV, resonant at 11565 eV) [3], while the field was switched between parallel and antiparallel orientation to the in-plane projection of the incident beam at every reflectivity angle. The degree of circular polarization was  $(88 \pm 1)\%$  as derived from a model for the performance of the phase-plates [4].

The fitting tool ReMagX [5] was used to evaluate the magnetic XRMR asymmetry ratio  $\Delta I = \frac{I_+ - I_-}{I_+ + I_-}$  plotted over the scattering vector  $q = \frac{4\pi}{\lambda} \sin \theta$ , where  $\lambda$ : wavelength,  $I_\pm$ : XRR intensity for different field directions and  $\theta$ : angle of incidence. The structural parameters (thickness, roughness) extracted from the fittings of the off-resonant XRR scans using literature values for the optical parameters  $\delta$  and  $\beta$ , are used to fit the resonant XRR curves and determine the optical parameters in resonance [6]. Afterwards, the XRMR asymmetry ratios are simulated using the previously derived parameters along with the variation of magneto-optic depth profiles for the magneto-optical parameters  $\Delta\delta$  and  $\Delta\beta$ . The ratio  $\frac{\Delta\beta}{\Delta\delta} = -14.3$  was kept fixed during fitting and was determined by adjusting the magneto-optical

data from the *ab initio* calculations to a fixed  $q$ -scan [3]. We calculated this ratio at an energy of 11565 eV where we also collected our XRM R measurements. Finally, by comparing the resulting  $\Delta\delta$  and  $\Delta\beta$  values to optical data from *ab initio* calculations [2], the magnetic moment per spin polarized Pt atom is identified.

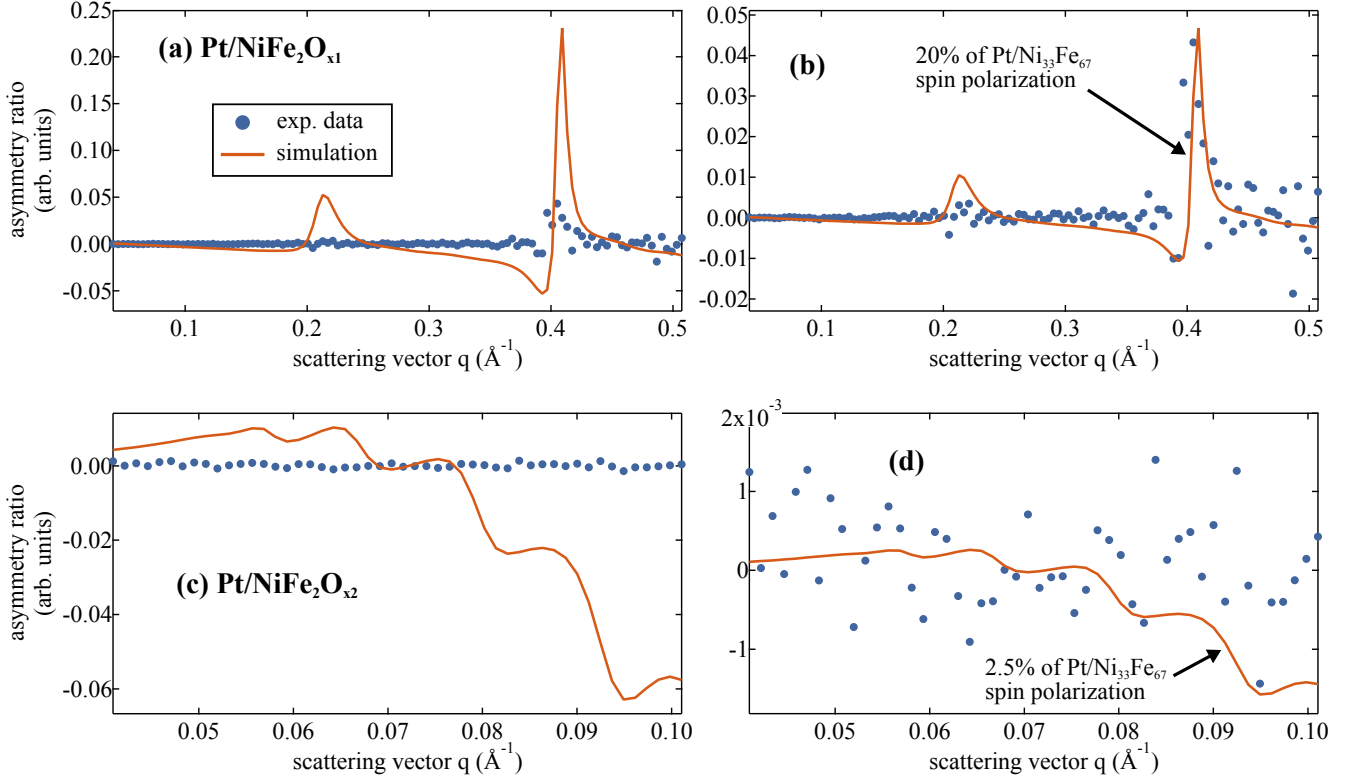

FIG. 1. (a) XRM R asymmetry ratio for Pt/NiFe<sub>2</sub>O<sub>x1</sub> and simulation using the magneto-optic depth profile of the Pt/Ni<sub>33</sub>Fe<sub>67</sub> bilayer, (b) assuming 20% of the Pt/Ni<sub>33</sub>Fe<sub>67</sub> spin polarization. (c) XRM R asymmetry ratio for Pt/NiFe<sub>2</sub>O<sub>x2</sub> and simulation using the magneto-optic depth profile of the Pt/Ni<sub>33</sub>Fe<sub>67</sub> bilayer, (d) assuming 2.5% of the Pt/Ni<sub>33</sub>Fe<sub>67</sub> spin polarization.

In Fig. 1 the measured XRM R asymmetry ratio is presented along with a simulation using a magneto-optic depth profile identical to the one derived for the Pt/Ni<sub>33</sub>Fe<sub>67</sub> bilayer for the Pt/NiFe<sub>2</sub>O<sub>x1</sub> (Fig. 1(a),(b)) and Pt/NiFe<sub>2</sub>O<sub>x2</sub> bilayers (Fig. 1(c),(d)), respectively. As in the case of the Pt/NFO analyzed in the letter, the simulated asymmetry ratio of the Pt/NiFe<sub>2</sub>O<sub>x1</sub> (Fig. 1(a)) deviates strongly from the one of the Pt/Ni<sub>33</sub>Fe<sub>67</sub> sample, although the same magneto-optic depth profile was used (Fig. 5(b) of the main manuscript), due to the different optical constants of Ni<sub>33</sub>Fe<sub>67</sub> and NiFe<sub>2</sub>O<sub>x1</sub>. Therefore, since the simulated asymmetry ratio of the Pt/NiFe<sub>2</sub>O<sub>x1</sub> sample does not match the experimental data, a potential MPE present in this film must be significantly smaller than in the all-metallic system. By decreasing the magnitude of the magneto-optic parameters down to 20% of the Pt/Ni<sub>33</sub>Fe<sub>67</sub> spin polarization (Fig. 1(b)), we can estimate a detection limit leading to an upper limit for the maximum magnetic moment in Pt of 0.1  $\mu_B$  per spin polarized Pt atom. Accordingly, for the Pt/NiFe<sub>2</sub>O<sub>x2</sub> bilayer we decreased the magnitude of the magneto-optic parameters down to 2.5% of the Pt/Ni<sub>33</sub>Fe<sub>67</sub> spin polarization (Fig. 1(d)) and we estimated a detection limit leading to an upper limit for the maximum magnetic moment in Pt of 0.01  $\mu_B$  per spin polarized Pt atom. The extracted limits for both samples are different compared to Pt/NFO due to different signal-to-noise ratios in the XRM R data.

### III. HEAT FLUX CALCULATION

To calculate the heat flux  $\phi_q$  in the IPM geometry we inserted Peltier elements as heat flux sensors right below the samples and converted the output signal of the sensor into heat flux by taking into account the cross section area of the heat between the sample and the Peltier element. We calibrated the heat flux sensors by using an electric heater resistor to simulate a Joule heat source as described by Sola *et al.* [7, 8]. In the OPM configuration, the heat flux was theoretically determined by taking into account the thermal conductivity of the FM layers. For the Pt/Ni<sub>33</sub>Fe<sub>67</sub> bilayer we additionally considered the contribution of the spin polarized layer of Pt with the effective spin polarized

thickness extracted from the XRMR investigations.

The heat  $Q$  which passes through every layer of the samples is calculated from

$$Q = \frac{\Delta T}{L_T} K \cdot S \quad (1)$$

where  $L_T$ : total length of the sample in the direction of the temperature gradient,  $S$ : side area perpendicular to the direction of the heat propagation and  $K$ : thermal conductivity of the corresponding layer. The  $\Delta T$  is extracted from the value of the thermal conductivity of the MAO substrate which is  $24 \text{ Wm}^{-1}\text{K}^{-1}$  [9] and the heat flux output taken from a Peltier element located below the substrate. We consider that the  $\Delta T$  remains the same along all the layers. The main contribution to the total heat of the sample comes from the MAO layer since this is the thickest part of every sample. However, we are only interested in the contribution of the FM layer in which the effects are generated. The thermal conductivities of the  $\text{NiFe}_2\text{O}_x$  ( $x > 0$ ) layers are assumed to be  $(8.5 \pm 0.9) \text{ Wm}^{-1}\text{K}^{-1}$  [10], since all of these samples are in the insulating regime at RT. The error is introduced since the absolute value of the thermal conductivity corresponds to a bulk material and not to thin films. Then the heat flux is determined from

$$\phi_q = \frac{K \Delta T}{L_T} \quad (2)$$

It is crucial to also consider the contribution of the spin polarized Pt layer to the heat flux in the case that an MPE is present. This has to be examined only for the  $\text{Pt}/\text{Ni}_{33}\text{Fe}_{67}$  bilayer as confirmed by XRMR. In this case  $K_{\text{Ni}_{33}\text{Fe}_{67}}$  consists of two components

$$K_{\text{Ni}_{33}\text{Fe}_{67}} = K_e + K_{\text{ph}} \quad (3)$$

where  $K_e$ : thermal conductivity of free electrons and  $K_{\text{ph}}$ : thermal conductivity of phonons. The value of  $K_e$  is calculated from the Wiedemann-Franz law

$$K_e = L \sigma T \quad (4)$$

where  $\sigma$ : measured electrical conductivity at each temperature  $T$  and  $L = 2.44 \cdot 10^{-8} \text{ W}\Omega\text{K}^{-2}$  is the Lorentz constant. The value of  $K_{\text{ph}}$  is regarded to be equal to  $(8.5 \pm 0.9) \text{ Wm}^{-1}\text{K}^{-1}$ . The contribution from the 1.0 nm spin polarized layer of Pt is quantified to be 17% of the heat flux of the  $\text{Ni}_{33}\text{Fe}_{67}$  layer. The chosen heat flux values for the normalization of the measured voltage in Fig. 2 of the main text are comparable but not identical. However, the magnitude of the normalized signal will not be influenced by the choice of the heat flux value due to the linear interdependency between both the voltage and the heat flux.

#### IV. PHYSICAL CHARACTERISTICS OF THE SAMPLES

In the Table I the measured physical parameters of all samples are presented, where  $t_{\text{FM}}$ : thickness of the FM,  $t_{\text{Pt}}$ : thickness of the Pt layer,  $t_{\text{Pt}}^{\text{NM}}$ : thickness of the non-magnetic fraction of Pt,  $t_{\text{Pt}}^{\text{SP}}$ : thickness of the spin polarized fraction of Pt,  $\rho_{\text{FM}}$ : electrical resistivity of the FM (measured on the samples without Pt on top), and  $\rho_{\text{Pt}}$ : electrical resistivity of Pt, for each film respectively. The  $\rho_{\text{Pt}}$  values were calculated from the measured  $\rho$  values of the twin samples with and without the Pt layer on top.

| Film                                    | Pt/NFO              | Pt/NiFe <sub>2</sub> O <sub>x1</sub> | Pt/NiFe <sub>2</sub> O <sub>x2</sub> | Pt/Ni <sub>33</sub> Fe <sub>67</sub> |
|-----------------------------------------|---------------------|--------------------------------------|--------------------------------------|--------------------------------------|
| $t_{\text{FM}}$ (nm)                    | 160                 | 60                                   | 35                                   | 10.4                                 |
| $t_{\text{Pt}}$ (nm)                    | 3.0                 | 2.7                                  | 3.1                                  | 3.5                                  |
| $t_{\text{Pt}}^{\text{NM}}$ (nm)        | 3.0                 | 2.7                                  | 3.1                                  | 2.5                                  |
| $t_{\text{Pt}}^{\text{SP}}$ (nm)        | 0.0                 | 0.0                                  | 0.0                                  | 1.0                                  |
| $\rho_{\text{FM}}$ ( $\Omega\text{m}$ ) | 40.5                | $1.5 \cdot 10^{-4}$                  | $4.5 \cdot 10^{-5}$                  | $4.2 \cdot 10^{-7}$                  |
| $\rho_{\text{Pt}}$ ( $\Omega\text{m}$ ) | $1.6 \cdot 10^{-7}$ | $1.7 \cdot 10^{-7}$                  | $1.8 \cdot 10^{-7}$                  | $1.6 \cdot 10^{-7}$                  |

TABLE I. Resistivity at room temperature and thickness for Pt/NFO, Pt/NiFe<sub>2</sub>O<sub>x1</sub>, Pt/NiFe<sub>2</sub>O<sub>x2</sub>, and Pt/Ni<sub>33</sub>Fe<sub>67</sub> samples.

Figure 2 represents the change of RT resistivity according to the partial O<sub>2</sub> pressure during deposition. The partial O<sub>2</sub> pressure was calculated from the partial Ar pressures and total pressures recorded during the deposition of each sample. A clear increase of the resistivity is observed when the amount of oxygen increases.

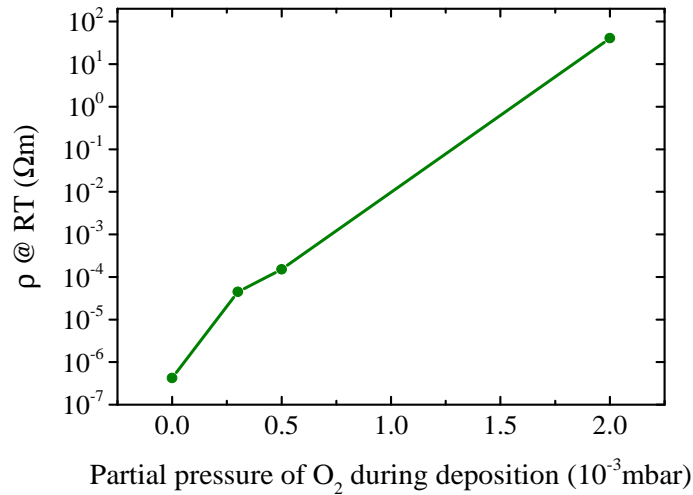

FIG. 2. Resistivity measured at RT for the corresponding partial O<sub>2</sub> pressure of all samples.

## V. BANDGAP ENERGY DETERMINATION

The optical band gap energies are obtained from ultraviolet-visible spectroscopy, and in that respect extracted using Tauc plots [1] ( $(\alpha E)^{0.5}$  versus energy), where  $\alpha(E)$  is the absorption coefficient extracted from the measured transmission  $T$  and reflectance  $R$  spectra by  $\alpha = \frac{1}{d} \ln \frac{1-R}{T}$ , where  $d$  is the thickness of the corresponding NiFe<sub>2</sub>O<sub>x</sub> ( $x > 0$ ) layer. The optical band gap for the NFO film is estimated to be  $E_{\text{gap}}^{\text{NFO}} \approx 1.49$  eV, close to our previous investigations [1], although the use of Tauc plots to determine the energy of a direct band gap in case of NFO can be erroneous [11]. The optical bandgap for the NiFe<sub>2</sub>O<sub>x<sub>1</sub></sub> and NiFe<sub>2</sub>O<sub>x<sub>2</sub></sub> sample is  $E_{\text{gap}}^{\text{NiFe}_2\text{O}_{x_1}} \approx 1.27$  eV and  $E_{\text{gap}}^{\text{NiFe}_2\text{O}_{x_2}} \approx 1.09$  eV, respectively, unveiling the more conducting character of the latter. A detailed band gap analysis on these NiFe<sub>2</sub>O<sub>x</sub> ( $x > 0$ ) samples is reported in Ref. [12]. The electric band gap determined from an activated conduction is in the range of some 0.1 eV in accordance with previous publications [1, 13, 14].

- 
- [1] C. Klewe, M. Meinert, A. Boehnke, K. Kuepper, E. Arenholz, A. Gupta, J.-M. Schmalhorst, T. Kuschel, and G. Reiss, *J. Appl. Phys.* **115**, 123903 (2014).
  - [2] T. Kuschel, C. Klewe, J.-M. Schmalhorst, F. Bertram, O. Kuschel, T. Schemme, J. Wollschläger, S. Francoual, J. Stempfer, A. Gupta, M. Meinert, G. Götz, D. Meier, and G. Reiss, *Phys. Rev. Lett.* **115**, 097401 (2015).
  - [3] T. Kuschel, C. Klewe, P. Bougiatioti, O. Kuschel, J. Wollschläger, L. Bouchenoire, S. D. Brown, J. M. Schmalhorst, D. Meier, and G. Reiss, *IEEE Trans. Magn.* **52**, 4500104 (2016).
  - [4] L. Bouchenoire, S. D. Brown, P. Thompson, J. A. Duffy, J. W. Taylor, and M. J. Cooper, *J. Synchrotron Radiat.* **10**, 172 (2003).
  - [5] S. Macke and E. Goering, *J. Phys.: Condens. Matter* **26**, 363201 (2014).
  - [6] C. Klewe, T. Kuschel, J.-M. Schmalhorst, F. Bertram, O. Kuschel, J. Wollschläger, J. Stempfer, M. Meinert, and G. Reiss, *Phys. Rev. B* **93**, 214440 (2016).
  - [7] A. Sola, M. Kuepferling, V. Basso, M. Pasquale, T. Kikkawa, K. Uchida, and E. Saitoh, *J. Appl. Phys.* **117**, 17C510 (2015).
  - [8] A. Sola, P. Bougiatioti, M. Kuepferling, D. Meier, G. Reiss, M. Pasquale, T. Kuschel, and V. Basso, *arXiv:1701.03285* (2017).
  - [9] B. Schulz and M. Hoffmann, *High Temp. - High Pressures* **34**, 203 (2002).
  - [10] A. T. Nelson, J. T. White, D. A. Andersson, J. A. Aguiar, K. J. McClellan, D. D. Byler, M. P. Short, and C. R. Stanek, *J. Am. Ceram. Soc.* **97**, 1559 (2014).
  - [11] M. Meinert and G. Reiss, *J. Phys.: Condens. Matter* **26**, 115503 (2014).
  - [12] P. Bougiatioti, O. Manos, C. Klewe, D. Meier, J.-M. Schmalhorst, T. Kuschel, and G. Reiss, in preparation (2017).
  - [13] H. Lord and R. Parker, *Nature* **188**, 929 (1960).
  - [14] D. Meier, T. Kuschel, L. Shen, A. Gupta, T. Kikkawa, K. Uchida, E. Saitoh, J.-M. Schmalhorst, and G. Reiss, *Phys. Rev. B* **87**, 054421 (2013).
